# Supplementary material for: Entropy-driven impurity-induced nematic-isotropic transition of liquid crystals
Source: arXiv:1910.05628 source file (2019-10-12)
Supplement: Supplementary file 1 [file Supplemental_Material.pdf]

## Supplemental Material
## to

# Entropy-driven impurity-induced nematic-isotropic transition of liquid crystals

Pritam Kumar Jana, Julien Lam, Nagma Parveen, Mikko J Alava, and Lasse Laurson

## Force field

For 4-cyano-4-hexylbiphenyl (6CB) liquid crystals the force field has the following functional form

$$E_f = E_{stretching} + E_{bending} + E_{torsional} + E_{vdw} + E_{electrostatic} \tag{1}$$

where

$$E_{stretching} = \sum_{bonds} \frac{1}{2} k_l (l - l_0)^2 \tag{2}$$

$$E_{bending} = \sum_{angles} \frac{1}{2} k_\theta (\theta - \theta_0)^2 \tag{3}$$

$$E_{torsional} = \sum_{dihedrals} \left[\frac{1}{2} k_1 (1 + \cos\varphi_i) + \frac{1}{2} k_2 (1 - \cos 2\varphi_i) + \frac{1}{2} k_3 (1 + \cos 3\varphi_i) + \frac{1}{2} k_4 (1 - \cos 4\varphi_i)\right] \tag{4}$$

$$E_{vdw} = \sum_{i,j} 4\varepsilon_{ij} \left[\left(\frac{\sigma_{ij}}{\varepsilon_{ij}}\right)^{12} - \left(\frac{\sigma_{ij}}{\varepsilon_{ij}}\right)^{6}\right] \tag{5}$$

$$E_{electrostatic} = \sum_{i,j} \frac{1}{4\pi\epsilon_0} \frac{q_i q_j}{r_{ij}} \tag{6}$$

Here $k_l$, $k_\theta$, and $k_n$ are the force constants for bond stretching, bond angle bending, and torsional force rotations, respectively. $l_0$ and $\theta_0$ are the equilibrium bond lengths and angles, $\sigma_{ij}$ and $\varepsilon_{ij}$ are the collision distance at which $E_{vdw} = 0$ and potential well depth, respectively. $q_i$ is the atomic charge. $l$, $\theta$, and $\varphi$ are the bond lengths, bond angles, and torsional angles, respectively. Force field parameters used in the simulations are summarized below.

### Force field parameters for 6CB liquid crystals

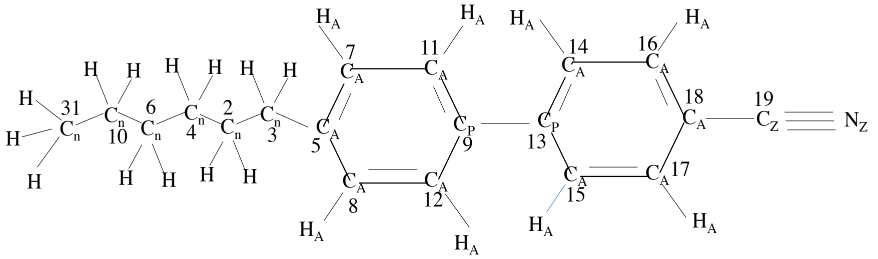

FIG. SM1. Structural details of 6CB molecule. All digits stand for the identity of the atoms. $C_A$ and $H_A$ are aromatic carbon and aromatic hydrogen. $C_P$ is the ring joining carbon atom. $C_n$ and H represent aliphatic carbon and hydrogen. $C_z$ and $N_z$ are the carbon and nitrogen from the cyano group. When we define the atoms using digits as suffix we consider $C_A$, $C_P$, $C_n$, $C_Z \equiv C$ or $H_A \equiv H$.

| Bond | $k_l$(eV Å$^{-2}$) | $l_0$(Å) |
|---|---|---|
| $C_A$-$H_A$ | 33.96 | 1.08 |
| $C_A$-$C_A$ | 44.32 | 1.38 |
| $C_A$-$C_P$ | 44.32 | 1.38 |
| $C_P$-$C_P$ | 27.28 | 1.47 |
| $C_A$-$C_Z$ | 31.52 | 1.31 |
| $C_Z$-$N_Z$ | 115.11 | 1.17 |
| $C_A$-$C_n$ | 24.47 | 1.50 |
| $C_n$-$C_n$ | 22.97 | 1.51 |
| $C_n$-HC | 31.65 | 1.09 |

Table 1. Bond stretching force constants ($\boldsymbol{k_l}$) and equilibrium bond lengths ($\boldsymbol{l_0}$)

| Angle | $k_\theta$($\times$ $10^{-5}$ eV/deg$^2$) | $\theta_0$(degree) |
|---|---|---|
| $C_A$-$C_A$-$H_A$ | 98.46 | 120 |
| $C_A$-$C_A$-$C_A$ | 84.94 | 120 |
| $C_A$-$C_P$-$C_P$ | 95.32 | 120 |
| $C_A$-$C_A$-$C_Z$ | 134.38 | 120 |
| $C_A$-$C_Z$-$N_Z$ | 71.10 | 180 |
| $C_n$-$C_n$-$C_n$ | 244.76 | 113 |
| $C_n$-$C_n$-HC | 116.98 | 112 |
| HC-$C_n$-HC | 147.25 | 107 |
| $C_n$-$C_A$-$C_A$ | 185.53 | 120 |
| $C_A$-$C_n$-HC | 92.466 | 109.5 |
| $C_A$-$C_n$-$C_n$ | 166.44 | 114 |

Table 2. Bond angle bending force constants ($\boldsymbol{k_\theta}$) and equilibrium bond angle ($\boldsymbol{\theta_0}$) for 6CB used in the simulations.

| Torsion | $k_1$($\times$ $10^{-2}$ eV) | $k_2$($\times$ $10^{-2}$ eV) | $k_3$($\times$ $10^{-2}$ eV) | $k_4$($\times$ $10^{-2}$ eV) |
|---|---|---|---|---|
| $C_A$-$C_A$-$C_A$-$C_A$ | 0.0 | 41.240011 | 0.0 | 0.0 |
| HC-$C_n$-$C_n$-$C_n$ | 0.0 | 0.0 | 0.16 | 0.0 |
| HC-$C_n$-$C_n$-HC | 0.0 | 0.0 | 0.14 | 0.0 |
| $C_A$-$C_P$-$C_P$-$C_A$ | 0.0 | 7.9 | 0.0 | 1.76 |
| $C_A$-$C_n$-$C_n$-$C_n$ | 3.04000011 | 0.03000016 | -0.1400002 | 0.54998707 |
| $C_n$-$C_n$-$C_n$-$C_n$ | 8.47 | 0.32 | 0.12 | -1.63 |
| $C_A$-$C_A$-$C_n$-$C_n$ | 0.0 | 3.59 | 0.0 | -0.29 |

Table 3. Torsional force constants ($\boldsymbol{k_1}, \boldsymbol{k_2}, \boldsymbol{k_3}, \boldsymbol{k_4}$) for LCs used in simulations.

| Atom | Charge (e) |
|---|---|
| Nz | -0.43 |
| $C_{19}$ | 0.395 |
| $C_{18}$ | 0.035 |
| $C_{14,15,16,17,11,12,7,8}$ | -0.122 |
| $C_{13,9,5}$ | 0 |
| $C_{2,3,4,6,10}$ | -0.12 |
| $C_{31}$ | -0.18 |
| $H_A$ | 0.122 |
| H | 0.06 |

Table 4. Partial charges for all atoms of 6CB molecule used in simulations.

| Atom | $\epsilon$ (eV) | $\sigma$ (Å) |
|---|---|---|
| Nz | 0.00737 | 3.200 |
| $C_{19}$ | 0.00651 | 3.650 |
| $C_{18}$ | 0.00304 | 3.550 |
| $C_{14,15,16,17,11,12,7,8}$ | 0.00304 | 3.550 |
| $C_{13,9,5}$ | 0.00304 | 3.550 |
| $C_{2,3,4,6,10}$ | 0.00286 | 3.500 |
| $C_{31}$ | 0.00286 | 3.500 |
| $H_A$ | 0.001306 | 2.420 |
| H | 0.001306 | 2.500 |

Table 5. $\boldsymbol{\varepsilon}$ and $\boldsymbol{\sigma}$ for all atoms of 6CB molecule used in simulations.

## Force field parameters for hexane

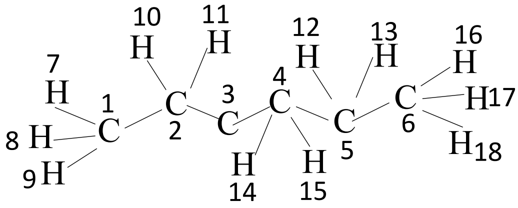

FIG. SM2. Chemical structure of hexane.

| Bond | $k_l$(eV Å$^{-2}$) | $l_0$(Å) |
|---|---|---|
| C-C | 23.2432 | 1.529 |
| C-H | 29.4876 | 1.090 |

Table 6. Bond stretching force constants ($\boldsymbol{k_l}$) and equilibrium bond lengths ($\boldsymbol{l_0}$).

| Angle | $k_\theta(\times 10^{-5}$ eV/deg$^2$) | $\theta_0$(degree) |
|---|---|---|
| C-C-C | 154.1546915 | 112.7 |
| C-C-H | 99.07376966 | 110.7 |
| H-C-H | 87.18150558 | 107.8 |

Table 7. Bond angle bending force constants ($\boldsymbol{k_\theta}$) and equilibrium bond angle ($\boldsymbol{\theta_0}$) for 6CB used in the simulations.

| Torsion | $k_1(\times 10^{-2}$ eV) | $k_2$ ($\times 10^{-2}$ eV) | $k_3$ ($\times 10^{-2}$ eV) | $k_4(\times 10^{-2}$ eV) |
|---|---|---|---|---|
| C-C-C-C | 7.54536 | -0.68081661 | 1.209859 | 0.00 |
| H-C-C-H | 0.000 | 0.000 | 1.378979 | 0.000 |
| H-C-C-C | 0.000 | 0.000 | 1.587127 | 0.000 |

Table 8. Torsional force constants ($\boldsymbol{k_1, k_2, k_3, k_4}$) for hexane used in simulations.

| Atom | Charge (e) |
|---|---|
| $C_{1,6}$ | -0.18 |
| $C_{2,3,4,5}$ | -0.12 |
| H | 0.06 |

Table 9. Partial charges for all atoms of hexane molecule used in simulations.

| Atom | $\epsilon$ (eV) | $\sigma$ (Å) |
|---|---|---|
| C | 0.002862032 | 3.50 |
| H | 0.00130092 | 2.50 |

Table 10. $\boldsymbol{\varepsilon}$ and $\boldsymbol{\sigma}$ for all atoms of hexane molecule used in simulations.

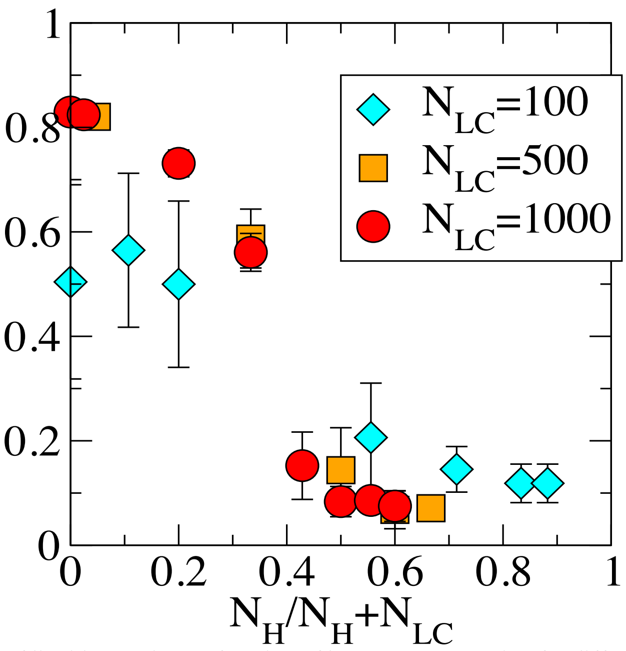


FIG. SM3. Order parameters of liquid crystals as a function of hexane concentration for different number of liquid crystals.

**Materials and Methods**

4′-Pentyl-4-biphenylcarbonitrile (5CB, liquid crystal, nematic, 98% pure, M.W.=249.357 g) and Nile blue chloride (dye content 85%) were purchased from Sigma-Aldrich. 5CB is milky white liquid at room temperature (about 26$^{o}$C) with a mass-density of 1.01 g/cm$^3$. It becomes a clear liquid at about 37$^{o}$C which is the phase transition (nematic to isotropic) temperature of 5CB. n-Hexane (98%, spectroscopy grade, mass-density 0.655 g/cm$^3$, M.W.=86.18 g) was purchased from Acros Organics. A freshly prepared solution of 0.1 mg/ml nile blue was used a stock solution, and further diluted to $10^{-3}$mg/ml in 5CB for all spectroscopy experiments. Nile blue was well soluble in 5CB at $10^{-3}$mg/ml. Ultrapure water (Millipore) of was used experiments of 5CB mixed with water.

Steady state fluorescence spectra (excitation and emission) were acquired employing a FLS 980 (Edinburgh Photonics which is equipped with 450 W ozone-free xenon arc lamp (excitation range 230 to 800 nm) and a single photon counting photomultiplier detector. The fluorescence emission was measured at a front face mode of the instrument to decrease the path length of emitted light and thereby avoid detection of scattered light from turbid 5CB. 300 μl of 5CB in disposable UV-Visible PMMA cuvettes (BioRad) was used in all our measurements. A flow cell holder was used to circulate water at specific temperature around the cuvette and maintain the temperature of the sample. Using a water bath, the temperature of the circulating water around the sample was controlled from 25 ºC to 42 ºC. The sample was equilibrated from 1-2 minutes at specified temperature prior to spectral acquisition. For experiments with hexane and water in 5CB, sample temperature was maintained at around 25 ºC.

Nile blue in 5CB at both nematic and disordered state has an absorption peak at about 525 nm. Therefore, the dye was excited at 525 nm in all our measurements using a bandwidth of 2.5 nm and the fluorescence emission was recorded between 550 to 750 nm using a bandwidth of 2.5 nm. The integration time of the spectral acquisition was 0.1 s and a step-size of 1 nm.
